# Supplementary material for: Krylov-projected quantum Monte Carlo
Source: arXiv:1409.2420 ancillary file (2015-06-03)
Supplement: Supplementary file 1 [file supp_material.pdf]

# Supplementary material for “Krylov-projected quantum Monte Carlo”

N. S. Blunt*
*University Chemical Laboratory, Lensfield Road, Cambridge, CB2 1EW, United Kingdom*

Ali Alavi
*University Chemical Laboratory, Lensfield Road, Cambridge, CB2 1EW, United Kingdom and Max Planck Institute for Solid State Research, Heisenbergstraße 1, 70569 Stuttgart, Germany*

George H. Booth†
*Department of Physics, King's College London, The Strand, London, WC2R 2LS, U.K.*
(Dated: May 20, 2015)

## SOLVING THE NON-ORTHONORMAL EIGENVALUE PROBLEM

The procedure in the main text describes a method of setting up a non-orthonormal eigenvalue problem, where the overlap matrix, $\boldsymbol{S}$, and projected Hamiltonian matrix, $\boldsymbol{T}$ are unbiased. Thus, as further averaging is performed, the exact eigenvalue problem is approached. The non-orthonormal eigenvalue problem is

$$\boldsymbol{Tx} = \epsilon \boldsymbol{Sx}. \tag{1}$$

We solve this problem using a canonical Löwdin orthogonalization procedure whereby the problem is transformed to

$$\boldsymbol{W}^T \boldsymbol{TWy} = \epsilon \boldsymbol{y}, \tag{2}$$

where

$$\boldsymbol{W} = \boldsymbol{UD}^{-1/2} \quad \text{and} \quad \boldsymbol{S} = \boldsymbol{UDU}^T. \tag{3}$$

This eigenvalue problem is then solved exactly by standard methods.

We note that spurious eigenvalues sometimes appear in the spectrum well below the ground-state energies. This is because the stochastic error on high-energy eigenvalues can often become very large, and sometimes so large that the eigenvalues appear below the ground-state eigenvalues, which typically have a very small stochastic error. These spurious poles are easily identified and removed. Apart from being significantly below other ground-state estimates, they are typically identifiable from their corresponding transition amplitude, which is very different to that of the ground state. We note that spurious eigenvalues are also often found in deterministic dynamical Lanczos approaches, although these appear due to numerical, rather than stochastic, instabilities[1–3].

* nsb37@cam.ac.uk
† george.booth@kcl.ac.uk

## SCALING IN THE REPLICA SAMPLING APPROACH

Setting up unbiased subspace Hamiltonian and overlap matrices requires the use of replica sampling, as described in the main text. The calculation of the overlap matrix is performed by

$$S_{ij} = (\boldsymbol{q}_i^{1\dagger} \boldsymbol{q}_j^2 + \boldsymbol{q}_i^{2\dagger} \boldsymbol{q}_j^1)/2. \tag{4}$$

This leads to a concern that when the number of walkers, $N_w$, is much smaller than the Hilbert space dimension, $D$, the overlaps, $\boldsymbol{q}_i^{1\dagger} \boldsymbol{q}_j^2$ and $\boldsymbol{q}_i^{2\dagger} \boldsymbol{q}_j^1$, will tend to 0. Indeed, for a wave function with uniform amplitudes, in the limit $D \gg N_w$ (where each basis state is occupied with probability $N_w/D$) the overlap will be approximately equal to $N_w^2/D$, and so quickly tends to 0 with increasing $D$. This would lead to large relative errors in the overlap matrix and statistically poor results, since the transformed Hamiltonian in Eq. 2 depends inversely on the overlap matrix eigenvalues.

Therefore, to demonstrate that a significant overlap between replicas *can* be achieved for systems of interest, even in the $D \gg N_w$ limit, we consider the quantity

$$S_{\text{replica}} = \frac{\boldsymbol{q}^{1\dagger} \boldsymbol{q}^2}{\sqrt{(\boldsymbol{q}^{1\dagger} \boldsymbol{q}^1)(\boldsymbol{q}^{2\dagger} \boldsymbol{q}^2)}}, \tag{5}$$

(i.e., the normalised replica overlap), where $\boldsymbol{q}$ represents the ground-state wavefunction (where the overlap between replicas will usually be smallest). In the limit of exact sampling this quantity will tend to 1, whereas it tends to 0 as the sets of determinants instantaneously occupied in the two replicas become disjoint. We consider this quantity as the system size increases, but with all other simulation parameters, including the total number of walkers in each replica, held constant.

In Figure 1 we present the scaling of $S_{\text{replica}}$ for the uniform electron gas with 14 electrons, in a plane wave basis set, as the number of plane waves ($M$) is increased. $10^6$ walkers were used in each case, and space sizes range from $\mathcal{O}[10^9 - 10^{19}]$, taking us well into the $D \gg N_w$ regime where one might expect $S_{\text{replica}}$ to scale as $D^{-1}$. In fact,

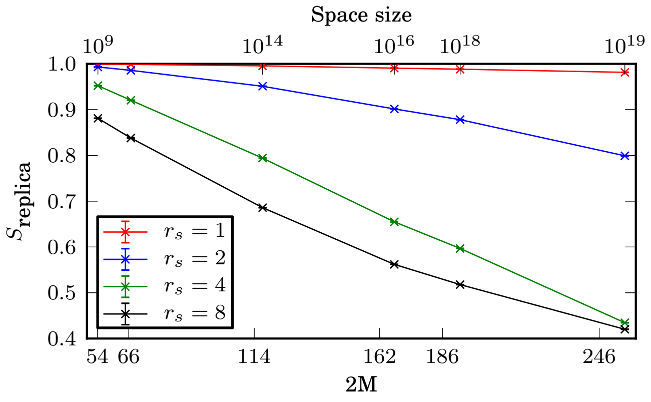


FIG. 1. The scaling of $S_{\rm replica}$ for the uniform electron gas, with 14 electrons, as the number of spin orbitals in the basis ($2M$) is increased. Only $10^6$ walkers were used in each case, and all simulation parameters (such as time step) were kept constant within each curve shown. The space size (to the nearest order of magnitude) is shown on the upper x-axis. As expected, the overlap between replicas decays more quickly for large values of $r_s$, where the wave function is more multi-configurational. However, the overlap between replicas remains large, even for space sizes well beyond the reach of traditional Lanczos. For $r_s = 4$, the overlap decreases roughly linearly with $M$, whereas the Hilbert space size increases factorially with $M$. Furthermore, the errorbars in this overlap are too small to be seen on the scale of this plot, indicating a stable sampling of the distributions.

the scaling is much less severe. For a density parameter ($r_s$) of 4, $S_{\rm replica}$ decreases approximately linearly with $M$ (whereas $D$ scales *factorially* with $M$). Regardless of the precise scaling, it is clear that $S_{\rm overlap}$ can remain significant, even for undersampled, highly non-trivial systems. A $S_{\rm overlap}$ value of 0.4 means that the equivalent contribution to the overlaps matrix will be 40% of the square of the walker population, which will usually be more than large enough for a statistically significant sampling of the desired expectation values.

In Figure 2 a similar scaling plot is presented, but for the one-dimensional Hubbard model at a filling fraction of 4/7, as the length is increased from 14 to 42 lattice sites. This covers Hilbert spaces sizes of $\mathcal{O}[10^5 - 10^{18}]$. Again, only $10^6$ walkers were used in each case. As found for the uniform electron gas model, significant ($> 0.1$) overlaps occur, even in the intermediate coupling regime, $U/t = 4$, for system sizes well into the substantially undersampled regime. The scaling of $S_{\rm overlap}$ with lattice size is slightly more severe than the scaling with basis set size for the uniform electron gas, but still much less severe than $1/D$. For much larger values of $U/t$, the decay of $S_{\rm replica}$ with system size will inevitably be more rapid. However, these results demonstrate that the use of replica sampling does not prevent statistically significant studies of systems well beyond the reach of the Lanczos method.

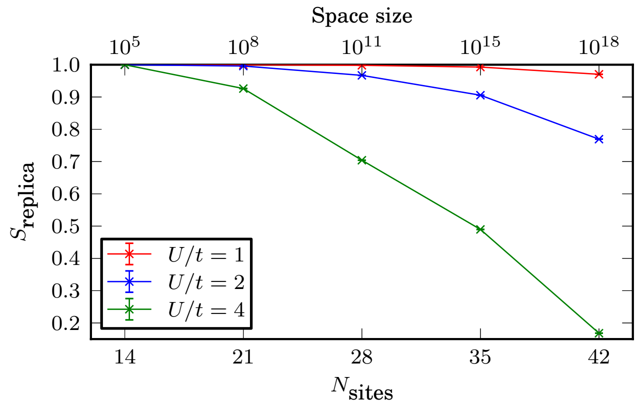


FIG. 2. The scaling of $S_{\rm replica}$ for the Hubbard model, at a filling fraction of 4/7. Only $10^6$ walkers were used in each case, and all simulation parameters were kept constant within each curve shown. The space sizes (to the nearest order of magnitude) are shown on the upper x-axis. As is found with the uniform electron gas results in Figure 1, the replica overlap decreases more quickly for more multi-configurational wave functions, but a significant overlap can be maintained even for some very large Hilbert space sizes in significantly correlated regimes.

The initiator method was used to produce figures 1 and 2, with an intiator threshold of $n_a = 3.0$ in both cases. Although most calculations are well converged with respect to initiator error, larger calculations with greater $U/t$ and $r_s$ values may not be fully converged with respect to the total energy, although this does not affect the validity of the results for $S_{\rm replica}$.

## THE HUBBARD MODEL

All results for the Hubbard model are defined with the Hamiltonian

$$\hat{H} = -t \sum_{\langle i,i' \rangle, \sigma} (\hat{c}^\dagger_{i,\sigma} \hat{c}_{i',\sigma} + \hat{c}^\dagger_{i',\sigma} \hat{c}_{i,\sigma}) + U \sum_i \hat{n}_{i,\uparrow} \hat{n}_{i,\downarrow}. \quad (6)$$

This system has a sign problem which increases in severity as $U/t$ increases[4, 5].

Calculations were performed in the $k$-space representation.

Results presented in Figure 2 of the main text were performed on an 18-site lattice at half filling. The lattice used is presented in Figure 3.

## BIAS IN DYNAMICAL CORRELATION FUNCTIONS

Results were presented in the main text for single particle Green functions. Here we plot the individual spectra for all 10 repeats of the results presented (for a 14-site

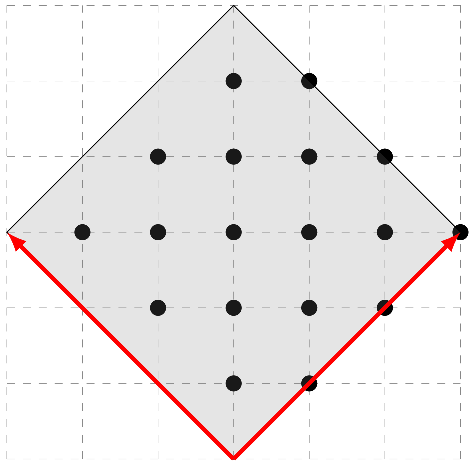

FIG. 3. 18-site lattice used for figure 2 of the main text.

Hubbard model at $U/t = 2$, with $\hat{V} = \hat{A} = \hat{c}^{\dagger}_{k\downarrow}$), in order to show the deviation between the results and potential bias in the eigenvalue estimates. In particular, we show the band structure at specific sampling points in the Brillouin zone, at $k = 5\pi/7$ and $k = 6\pi/7$.

In Figure 4 results are shown for $k = 5\pi/7$. It is seen that the lowest two poles, which both have large transition amplitudes, are captured very accurately by KP-FCIQMC. However, a larger stochastic error and a noticeable bias to higher frequency is present for the next highest pole. While the stochastic error in the result will account for some of the discrepancy, any systematic shifting of the peak is due to a bias in the non-linear diagonalization step. We emphasize that both the stochastic noise and systematic bias in these results is expected to decrease as the number of walkers increases, improving the accuracy by which the $\boldsymbol{S}$ and $\boldsymbol{T}$ matrices are sampled. Furthermore, increased averaging over independent runs will also reduce both the systematic and stochastic error in the matrices and eigenvalues, assuming that other systematic errors such as initiator error are negligible (which itself can be reduced by increasing walker number).

Figure 5 presents similar results for $k = 6\pi/7$. Again, the lowest-energy poles are captured well, but the next three peaks are merged into only two poles in the KP-FCIQMC results. This can happen with several eigenvalues which are close in energy.

These results are in line with the conclusions in the main text, that KP-FCIQMC is good at calculating relatively low-energy poles with large transition amplitudes, while the accuracy will degrade with sampling of higher frequencies and smaller transition amplitudes.


[1] Z. Bai, J. Demmel, J. Dongarra, A. Ruhe, and H. van der Vorst, *Templates for the Solution of Eigenvalue Problems: A Practical Guide* (SIAM, Philadelphia, 2000)

[2] J. Cullum and R. Willoughby, *Lanczos algorithms for large symmetric eigenvalue computations, Vol. 2* (Birkhäuser, Boston, 1985)

[3] P. E. Dargel, A. Woellert, A. Honecker, I. P. McCulloch, U. Schollwoeck, and T. Pruschke, Phys. Rev. B **85**, 205119 (2012)

[4] J. S. Spencer, N. S. Blunt, and W. M. C. Foulkes, J. Chem. Phys. **136**, 054110 (2012)

[5] J. J. Shepherd, G. E. Scuseria, and J. S. Spencer, Phys. Rev. B **90**, 155130 (2014)

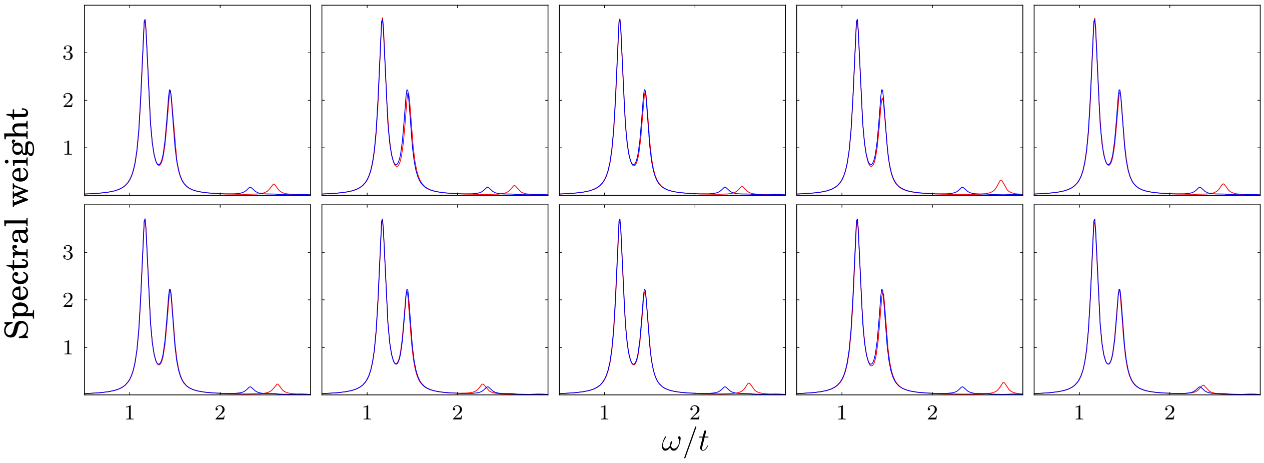


FIG. 4. 10 repeated KP-FCIQMC results, plotted against results from spectral Lanczos, with $\hat{V} = \hat{A} = \hat{c}^{\dagger}_{k\downarrow}$, where $k = 5\pi/7$. It can be seen that the two lower poles are always captured accurately. However the third pole, which has a much smaller transition amplitude (and therefore a smaller component in the sampled Krylov vectors) is less accurately captured. In particular, the KP-FCIQMC estimate of this eigenvalue is usually higher than the Lanczos estimate, suggesting a bias.

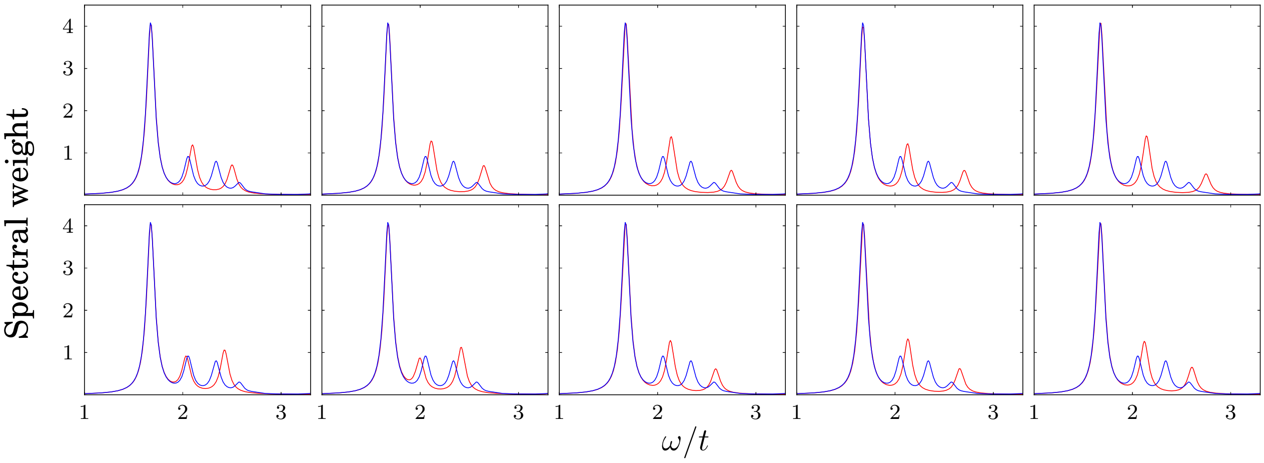


FIG. 5. 10 repeated KP-FCIQMC results, plotted against results from spectral Lanczos, with $\hat{V} = \hat{A} = \hat{c}^{\dagger}_{k\downarrow}$, where $k = 6\pi/7$. The lowest pole is captured accurately by KP-FCIQMC. However, the next three poles from Lanczos appear to always be merged into only two poles in our KP-FCIQMC results.
